# Supplementary material for: Rainy: Unlocking Satellite Calibration for Deep Learning in Precipitation
Source: arXiv:2504.10776 source file (2025-04-15)
Supplement: Supplementary file 1 [file X_suppl.tex]

% \clearpage
% \setcounter{page}{1}
% \setcounter{section}{0}
% \setcounter{table}{0}
% \setcounter{figure}{0}
% \renewcommand{\thetable}{A\arabic{table}}
% \renewcommand{\thefigure}{A\arabic{figure}}
% \maketitlesupplementary

% \appendix

\clearpage
\newpage
\appendix
\onecolumn
\setcounter{page}{1}
\setcounter{section}{0}
\setcounter{table}{0}
\setcounter{figure}{0}

% \maketitlesupplementary

\section{Data Preprocessing}
\label{sec_data_preprocessing}

This study utilizes two key data sources: \textbf{IMERG-Late} (Integrated Multi-satellite Retrievals for GPM - Late Run) and \textbf{CMPA} (China Meteorological Administration Precipitation Analysis). IMERG-Late data have a spatial resolution of 0.1 degrees and a temporal resolution of 30 minutes, whereas CMPA data have a higher spatial resolution of 0.05 degrees and a temporal resolution of 1 hour. To integrate these datasets for subsequent analysis, several preprocessing steps were carried out, including temporal and spatial alignment, upscaling, calibration, and data saving.

\subsection{Temporal Alignment}

Given the difference in temporal resolutions between IMERG-Late (30 minutes) and CMPA (1 hour), the first step involved aligning the time steps. In this study, the CMPA data were temporally interpolated from a 1-hour time step to a 30-minute resolution to match the IMERG-Late data. Linear interpolation was used to ensure temporal consistency between the two datasets, making them suitable for joint analysis.

\subsection{Spatial Upscaling}

The spatial resolution of IMERG-Late data is 0.1 degrees, while CMPA has a finer spatial resolution of 0.05 degrees. To handle this discrepancy, the CMPA data were downscaled to a coarser resolution of 0.1 degrees to match the IMERG-Late grid. This spatial upscaling was performed using linear interpolation, ensuring that the two datasets are spatially consistent. This process facilitated the integration of CMPA data with IMERG-Late data for further analysis, enabling comparisons at the same spatial resolution.

\subsection{Data Cropping and Saving}

The cropping process involves traversing each time data to identify monitoring stations and selecting the $256 \times 256$ pixel area that covers the maximum number of stations. This method ensures that each cropped tile contains the highest possible density of monitoring stations, optimizing data representation for model training.

The cropped data were saved in four formats:\\
\textbf{PNG Format}: The cropped data were stored in PNG format, primarily for visualization and model training. PNG provides a high compression rate with lossless quality, making it suitable for large-scale data storage and fast read access during model development. \\
\textbf{TIF Format}: To preserve the geographic information, the cropped data were also saved in GeoTIFF format. TIF files can retain high-quality imagery and embed geographic reference information, which is essential for subsequent spatial analysis and Geographic Information System (GIS) applications.\\
\textbf{NPY Format}: The data were also saved in NPY format, a binary file format used by NumPy, which allows fast and efficient access to arrays, making it suitable for machine learning tasks that require rapid data loading.\\
\textbf{NPZ Format}: To enable compressed storage of multiple arrays, the data were saved in NPZ format, which is a compressed archive of NPY files. This format is efficient for storing large datasets and supports quick access to multiple arrays within a single file.

By storing the data in these four formats, we ensure that the spatial information remains intact while making the data easily accessible for machine learning, visualization, and spatial analysis tasks. The cropped tiles are ready for use in deep learning models, particularly in scenarios where large datasets are needed.

\subsection{Summary}

% version1
% Through these preprocessing steps, including temporal alignment, spatial upscaling, data calibration, and cropping, we successfully integrated the IMERG-Late and CMPA datasets. The processed data are well-prepared for subsequent precipitation analysis and machine learning model training. The dual-format saving (PNG and GeoTIFF) ensures that both machine learning and geospatial analysis applications can be effectively supported. This preprocessing workflow offers a robust foundation for the analysis and integration of multi-source precipitation datasets.

% version2
By applying these preprocessing steps—temporal alignment, spatial upscaling, and targeted cropping—we successfully integrated the IMERG-Late and CMPA datasets. The processed data are optimally prepared for subsequent precipitation analysis and machine learning model training. Saving the data in multiple formats (PNG, GeoTIFF, NPY, and NPZ) ensures compatibility with both machine learning applications and geospatial analysis, providing a flexible and comprehensive foundation for multi-source precipitation dataset analysis and integration.

\section{Evaluation Metrics}
\label{sec_metrics}

These are commonly used metrics in the field of satellite sensor calibration, as shown in Table \ref{table:metrics_appendix}.

$H$ represents the number of hit events, $M$ is the number of missed precipitation events, and $F$ is the number of false precipitation events. Typically, a threshold of 0.2 mm/h is used to determine whether precipitation has occurred. If both the satellite and ground observations detect precipitation of 0.2 mm/h or more, it is considered a hit precipitation event. If the ground detects precipitation of 0.2 mm/h or more, but the satellite does not, it is considered a missed precipitation event. If the satellite detects precipitation of 0.2 mm/h or more, but the ground does not, it is considered a false precipitation event. $S$ is the total precipitation observed by the satellite, $G$ is the total precipitation observed by the ground, and $n$ is the sample size. $S_H$ is the precipitation observed by the satellite during hit events, $G_H$ is the precipitation observed by the ground during hit events, $G_M$ is the precipitation observed by the ground during missed events, and $S_F$ is the precipitation observed by the satellite during false events. $\overline{G}$ is the mean ground precipitation, and $\overline{S}$ is the mean satellite precipitation.

\begin{table*}

    \caption{Some commonly used evaluation metrics in satellite calibration.}
    \centering
    \begin{tabular}{ccc}
    \toprule
        \textbf{Metrics} & \textbf{Equations} & \textbf{Perfect Value} \\ \midrule
        Probability of Detection (POD) & $H={H\over{H+M}}$ & 1 \\ 
        False Alarm Ratio (FAR) & $FAR={F\over{H+F}}$ & 0 \\ 
        Correlation Coefficient (CC) & $CC={\frac{\sum_{i=1}^{n} {{(G_{i}-\overline{{G}})}\,(S_{i}-\overline{S})}}{{\sqrt{\sum_{i=1}^{n}{{(G_{i}-\overline{G})}^{2}}}\times\sqrt{\sum_{i=1}^{n}{{({S}_{i}-\overline{S})}^{2}}}}}}$ & 1 \\ 
        Root Mean Squared Error (RMSE) & $RMSE=\sqrt{{\frac{1}{n}\sum_{i=1}^{n}(S_i-G_i)^2}}$ & 0 \\ 
        Normalized Mean Absolute Error (NMAE) & $NMAE=\frac{\sum_{i=1}^{n}{\lvert{S_i-G_i\lvert}}}{\sum_{i=1}^{n}{G_i}}$ & 0 \\ 
        Normalized RMSE (NRMSE) & $NRMSE={{\sqrt{{\frac{1}{n}\sum_{i=1}^{n}(S_i-G_i)^2}}}\over{\overline{G}}}$ & 0 \\ 
        Total Bias (TB) & $TB=\frac{\sum_{i=1}^{n}{(S_i-G_i)}}{\sum_{i=1}^{n}G_i}\times100\%$ & 0 \\ 
        Hit Bias (HB) & $HB=\frac{\sum_{i=1}^{n}{(S_{H_i}-G_{H_i})}}{\sum_{i=1}^{n}G}\times100\%$ & 0 \\ 
        Miss Bias (MB) & $MB=\frac{\sum_{i=1}^{n}{-G_{M_i}}}{\sum_{i=1}^{n}G}\times100\%$ & 0 \\ 
        False Bias (FB) & $FB=\frac{\sum_{i=1}^{n}{S_{F_i}}}{\sum_{i=1}^{n}G}\times100\%$ & 0 \\ \bottomrule
    \end{tabular}
    \label{table:metrics_appendix}
\end{table*}

\section{Precipitation Level}
\label{sec_level}

According to China’s latest precipitation classification standard (GB/T 28592-2012), precipitation is divided into six levels: light rain, moderate rain, heavy rain, storm rain, severe storm, and extraordinary storm. The specific details are shown in Table \ref{table_level}.

% table_level
\begin{table}
    \centering
    % \caption{Rainfall intensity classification description.}
    \caption{Precipitation level description. We selected the 24-hour version.}
    \begin{tabular}{cccc}
        \toprule
        \textbf{Level} & \textbf{Event} & \textbf{12-Hour (mm)} & \textbf{24-Hour (mm)} \\ 
        \midrule
        0&  No Rain        & $<$ 0.1          & $<$ 0.1           \\
        1&  Light Rain     & 0.1 $\sim$ 4.9   & 0.1 $\sim$ 9.9    \\ 
        2&  Moderate Rain  & 5.0 $\sim$ 14.9  & 10.0 $\sim$ 24.9  \\ 
        3&  Heavy Rain     & 15.0 $\sim$ 29.9 & 25.0 $\sim$ 49.9  \\ 
        4&  Storm Rain     & 30.0 $\sim$ 69.9 & 50.0 $\sim$ 99.9  \\ 
        5&  Severe Storm   & 70.0 $\sim$ 139.9 & 100.0 $\sim$ 249.9 \\ 
        6&  Extraordinary Storm & $\geq$ 140.0 & $\geq$ 250.0 \\ 
        \bottomrule
    \end{tabular}
    \label{table_level}
\end{table}

\section{Tables}

% table_kernel_ablation
\begin{table*}[!ht]
    \centering
    % \resizebox{0.9\linewidth}{!}{
    % \caption{Comparison of kernels across \textit{taper loss} for daily and hourly data. }
    \caption{Comparison of different kernel functions in \textit{Taper Loss} for daily and hourly data. \textbf{Bold} values indicate the best performance, while \underline{underlined} values represent the second-best results.}
    \resizebox{1.0\linewidth}{!}{
    \begin{subtable}[t]{\linewidth}
        \centering
        \caption{Daily data.}
        \begin{tabular}{c|ccc|ccc}
        \toprule
            \multirow{2}{*}{\textbf{Kernel Type}} & \multicolumn{3}{c|}{\bm{$\mathcal{L}_{Taper} + \mathcal{L}_1$}} & \multicolumn{3}{c}{\bm{$\mathcal{L}_{Taper} + \mathcal{L}_2$}} \\ \cline{2-7}
            ~ & \textbf{RMSE} & \textbf{MAE} & \textbf{R$^2$} & \textbf{RMSE} & \textbf{MAE} & \textbf{R$^2$} \\ \midrule
            Exponential & \textbf{0.1349±0.0049} & \underline{0.0468±0.0011} & \textbf{0.6339±0.0232} & \underline{0.1342±0.0024} & 0.0544±0.0021 & \underline{0.6368±0.011} \\ 
            Linear & 0.1361±0.0024 & \textbf{0.0467±0.0018} & 0.6286±0.0108 & 0.1348±0.003 & \underline{0.0516±0.0026} & 0.6344±0.0138 \\ 
            Power-law & 0.1391±0.0193 & 0.0486±0.0143 & 0.6149±0.1071 & 0.1412±0.0125 & 0.054±0.0146 & 0.6054±0.0657 \\ 
            Gaussian & \underline{0.1351±0.0032} & 0.0472±0.0019 & \underline{0.633±0.0145} & \textbf{0.133±0.0029} & \textbf{0.0499±0.0029} & \textbf{0.642±0.013} \\ \bottomrule
        \end{tabular}
    \end{subtable}
    }
    \resizebox{1.0\linewidth}{!}{
    \begin{subtable}[t]{\linewidth}
        \centering
        \caption{Hourly data.}
        \begin{tabular}{c|ccc|ccc}
        \toprule
            \multirow{2}{*}{\textbf{Kernel Type}} & \multicolumn{3}{c|}{\bm{$\mathcal{L}_{Taper} + \mathcal{L}_1$}} & \multicolumn{3}{c}{\bm{$\mathcal{L}_{Taper} + \mathcal{L}_2$}} \\ \cline{2-7}
            ~ & \textbf{RMSE} & \textbf{MAE} & \textbf{R$^2$} & \textbf{RMSE} & \textbf{MAE} & \textbf{R$^2$} \\ \midrule
            Exponential & \textbf{0.1174±0.0016} & \underline{0.0179±0.0012} & \textbf{0.3736±0.0179} & \textbf{0.1128±0.0004} & \textbf{0.0202±0.001} & \textbf{0.421±0.0042} \\ 
            Linear & 0.1184±0.0023 & 0.0176±0.001 & \underline{0.3629±0.0257} & \underline{0.1131±0.0005} & 0.0237±0.0011 & 0.4184±0.005 \\ 
            Power-law & 0.1199±0.0381 & 0.0176±0.0079 & 0.3464±0.0741 & 0.1132±0.0071 & 0.0207±0.0089 & 0.4174±0.0815 \\ 
            Gaussian & \underline{0.1189±0.002} & \textbf{0.0174±0.0011} & 0.357±0.0226 & \underline{0.1131±0.0007} & \underline{0.0219±0.0011} & \underline{0.4181±0.0075} \\ \bottomrule
        \end{tabular}
    \end{subtable}
    }
    \label{table_kernel_compare}
\end{table*}

\clearpage
\section{Figures}

% fig_alpha_daily
\begin{figure}[!ht]
    \centering
% row1
    \begin{minipage}{0.49\textwidth}
        \centering 
        \includegraphics[width=\textwidth]{icml2025/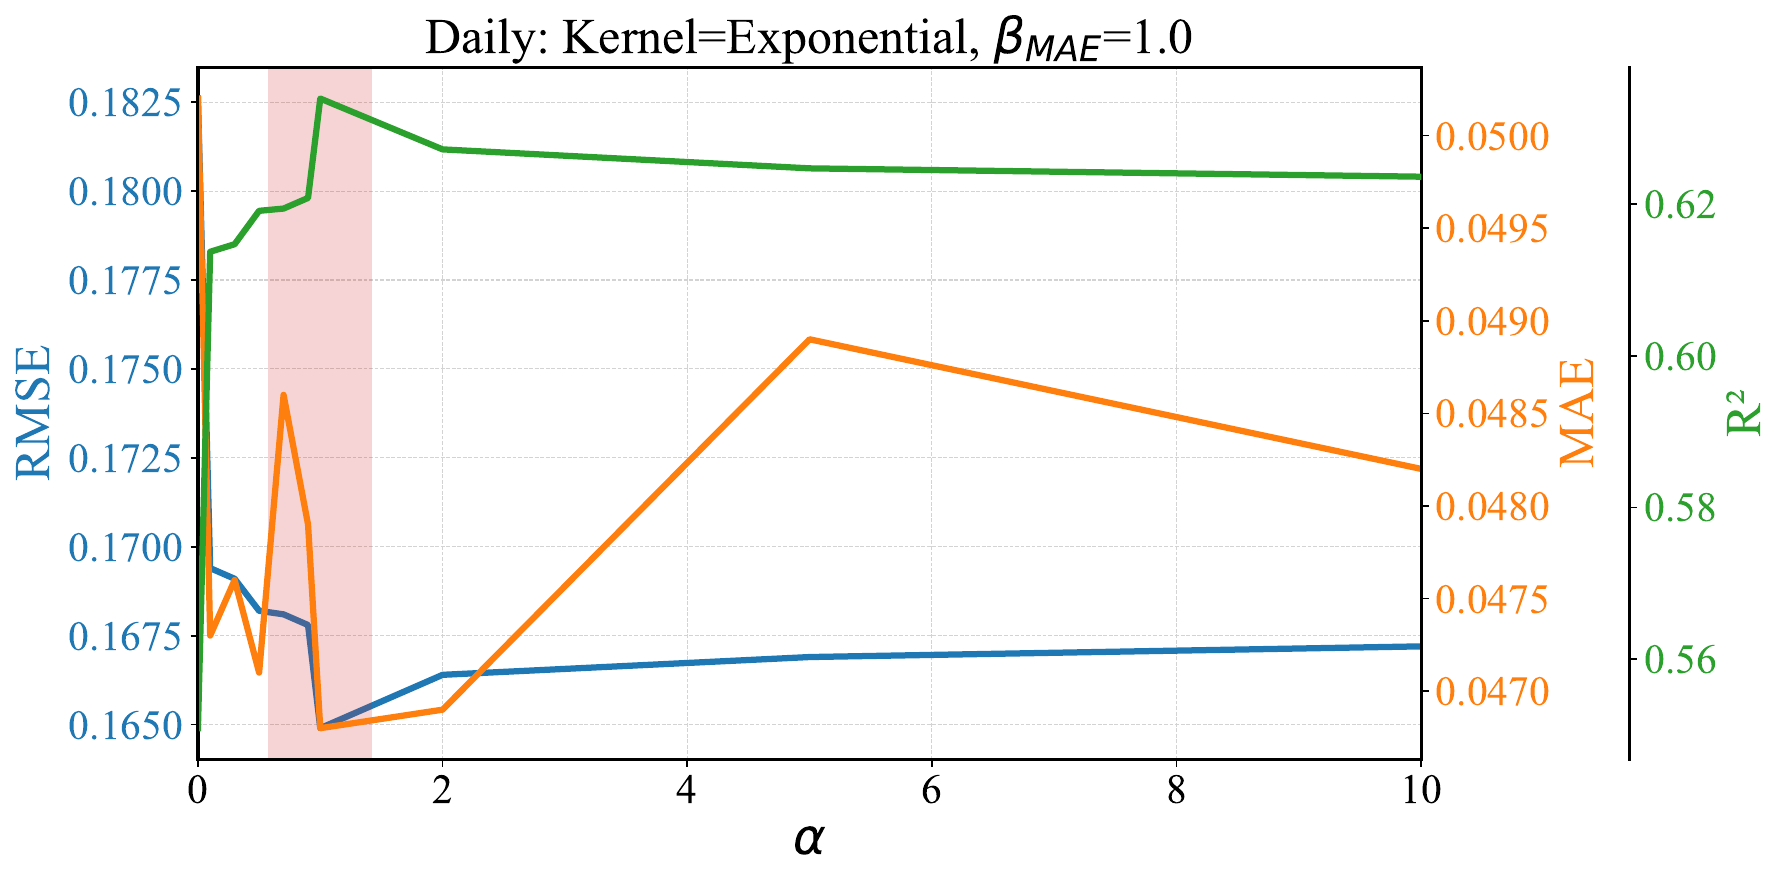}
    \end{minipage}
    \hspace{-6pt}
    \begin{minipage}{0.49\textwidth}
        \centering 
        \includegraphics[width=\textwidth]{icml2025/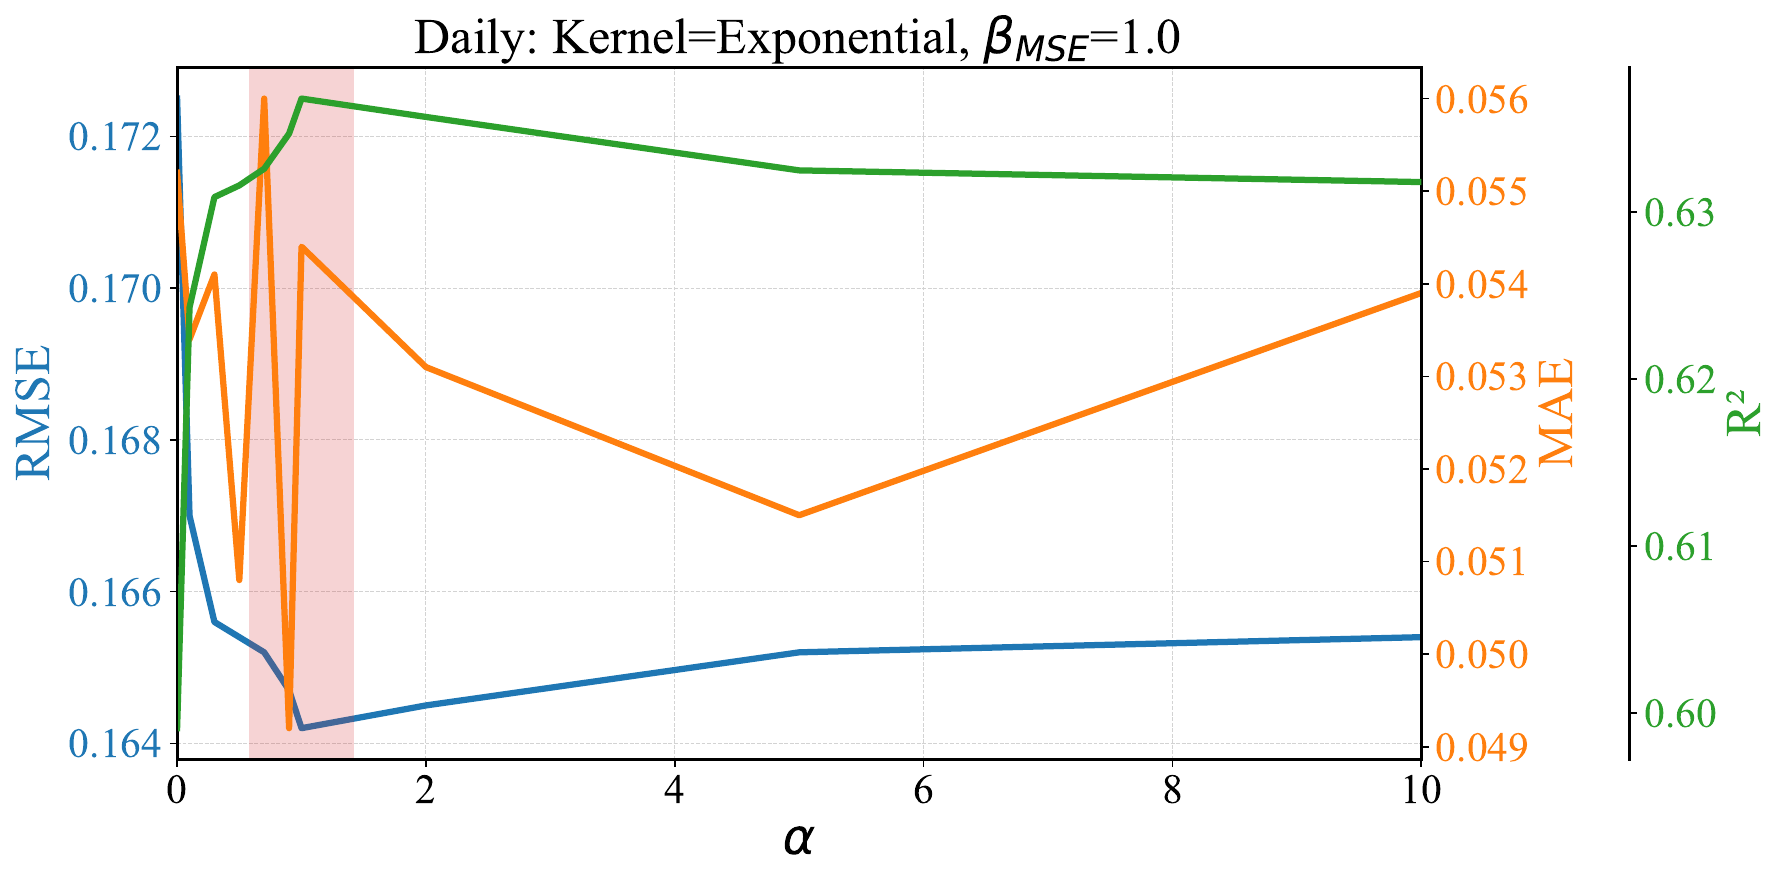}
    \end{minipage}
    \hspace{-6pt}
    \\
% row2
    \begin{minipage}{0.49\textwidth}
        \centering 
        \includegraphics[width=\textwidth]{icml2025/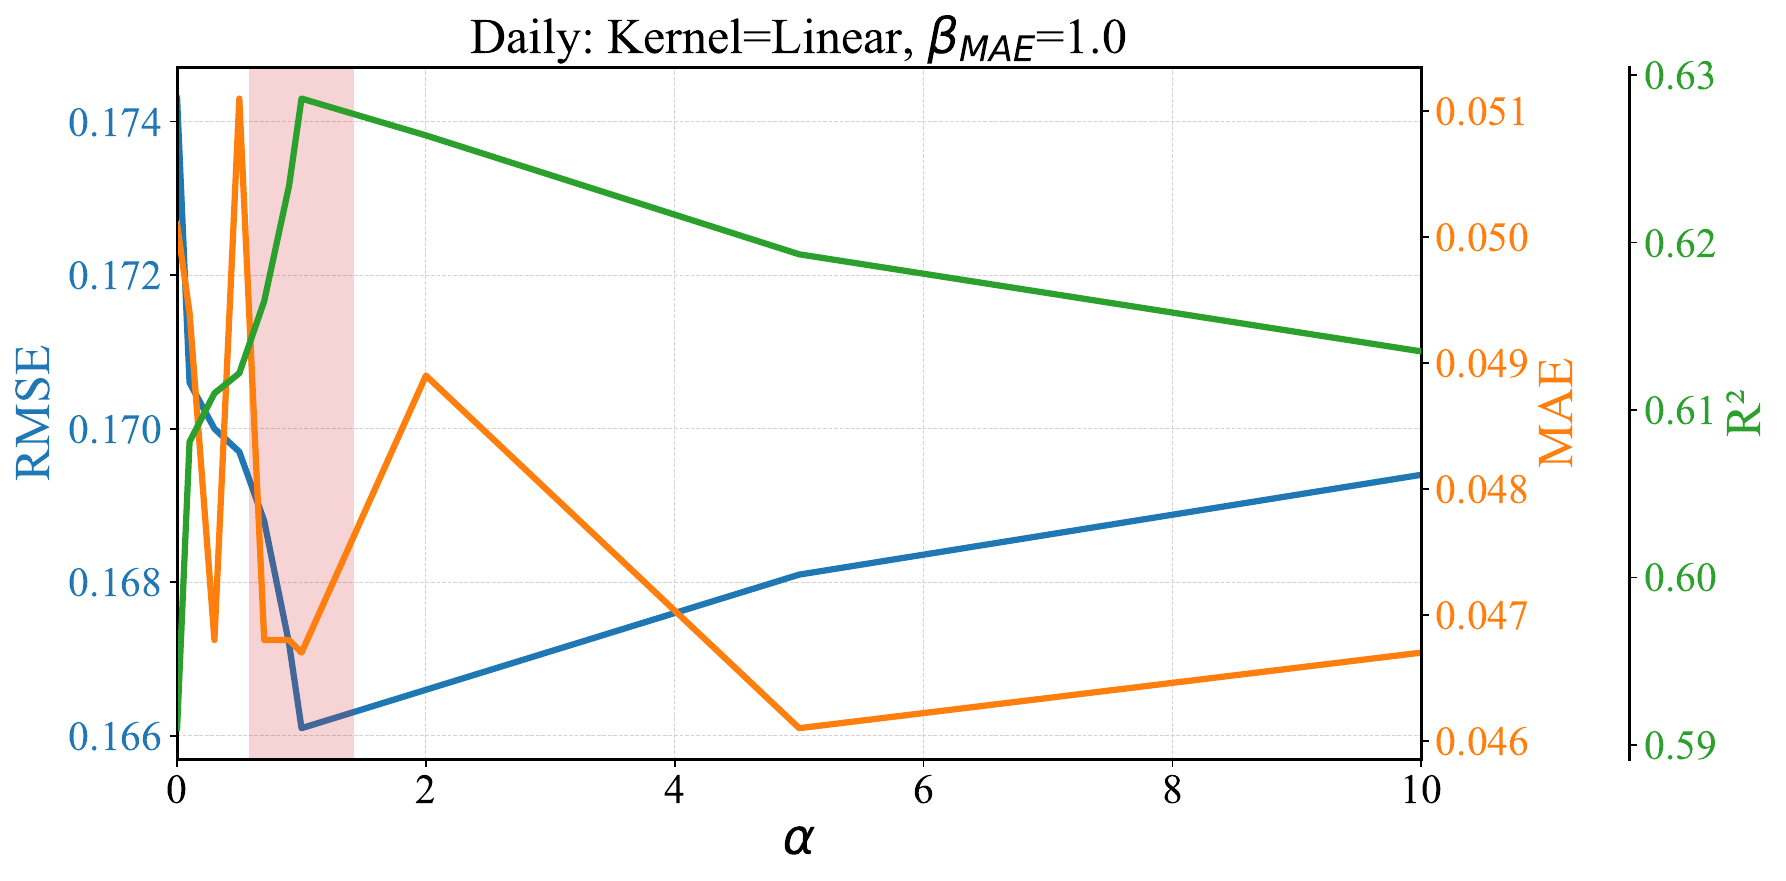}
    \end{minipage}
    % \hspace{-6pt}
    \begin{minipage}{0.49\textwidth}
        \centering 
        \includegraphics[width=\textwidth]{icml2025/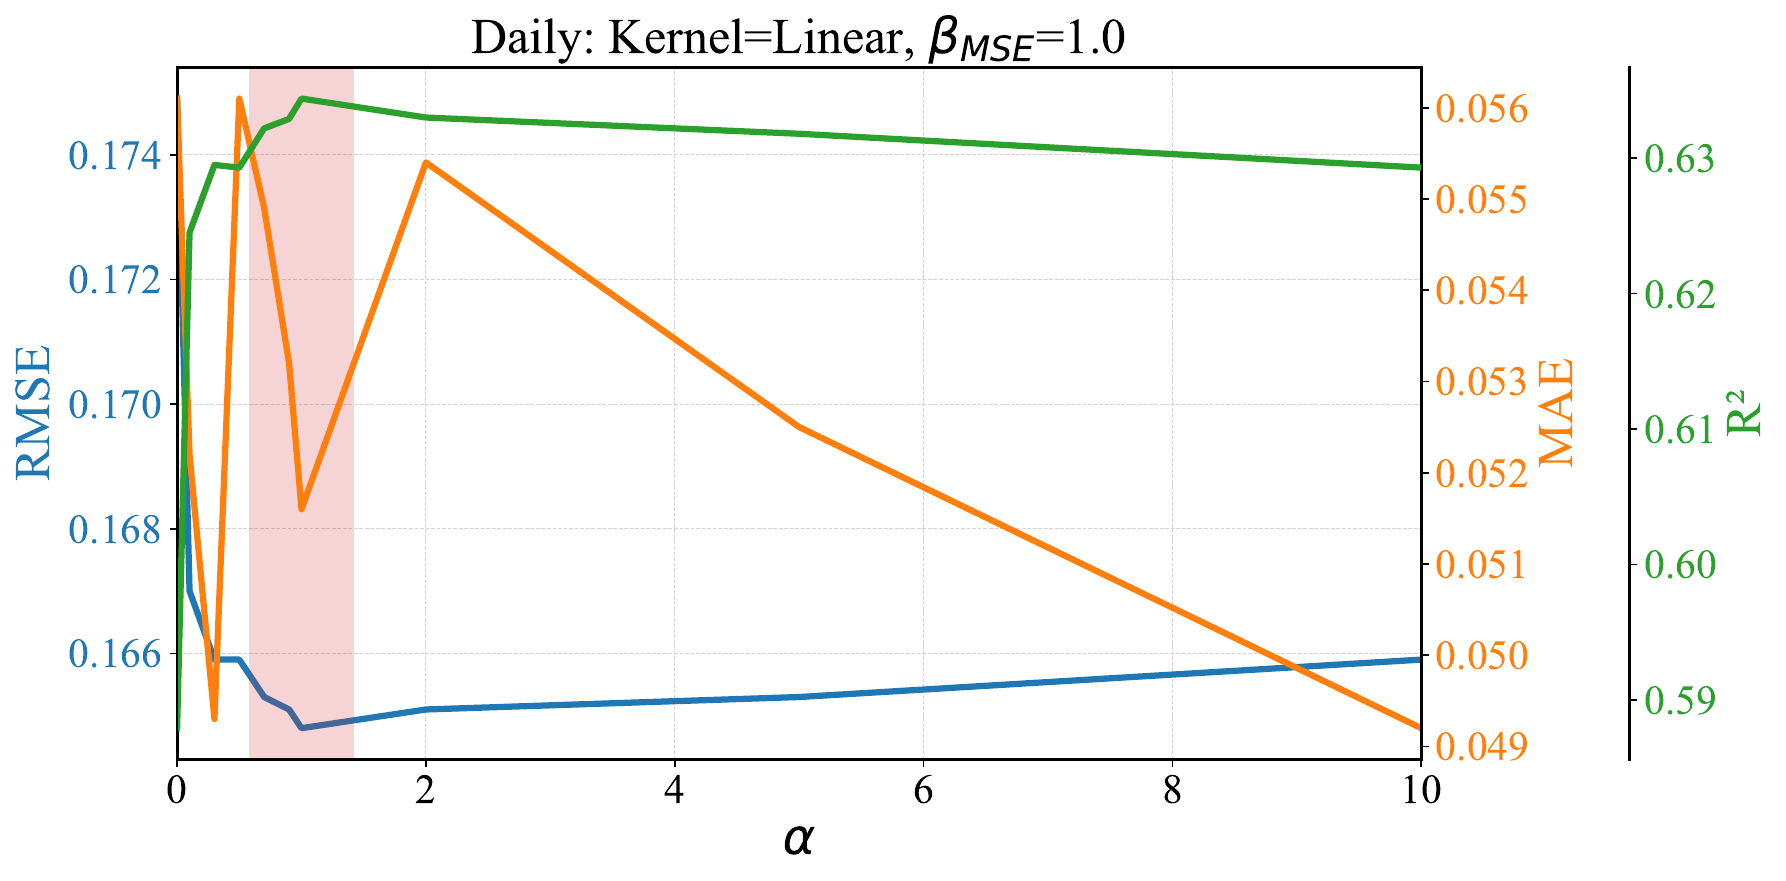}
    \end{minipage}
    \hspace{-6pt}
    \\
% row3
    \begin{minipage}{0.49\textwidth}
        \centering 
        \includegraphics[width=\textwidth]{icml2025/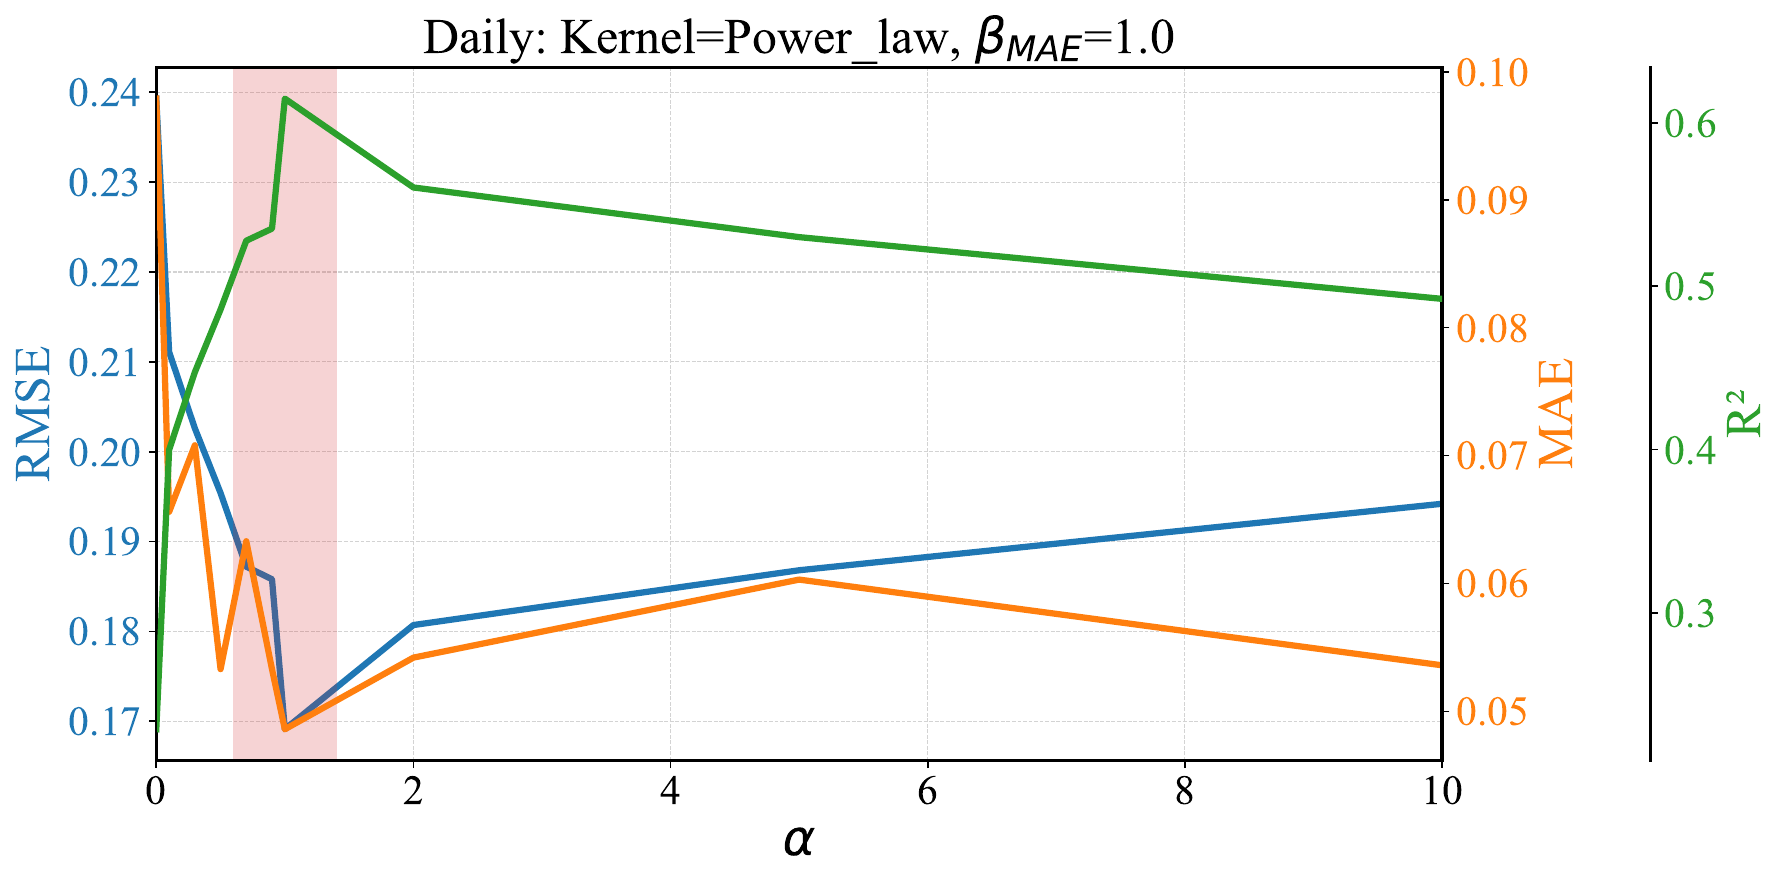}
    \end{minipage}
    \hspace{-6pt}
    \begin{minipage}{0.49\textwidth}
        \centering 
        \includegraphics[width=\textwidth]{icml2025/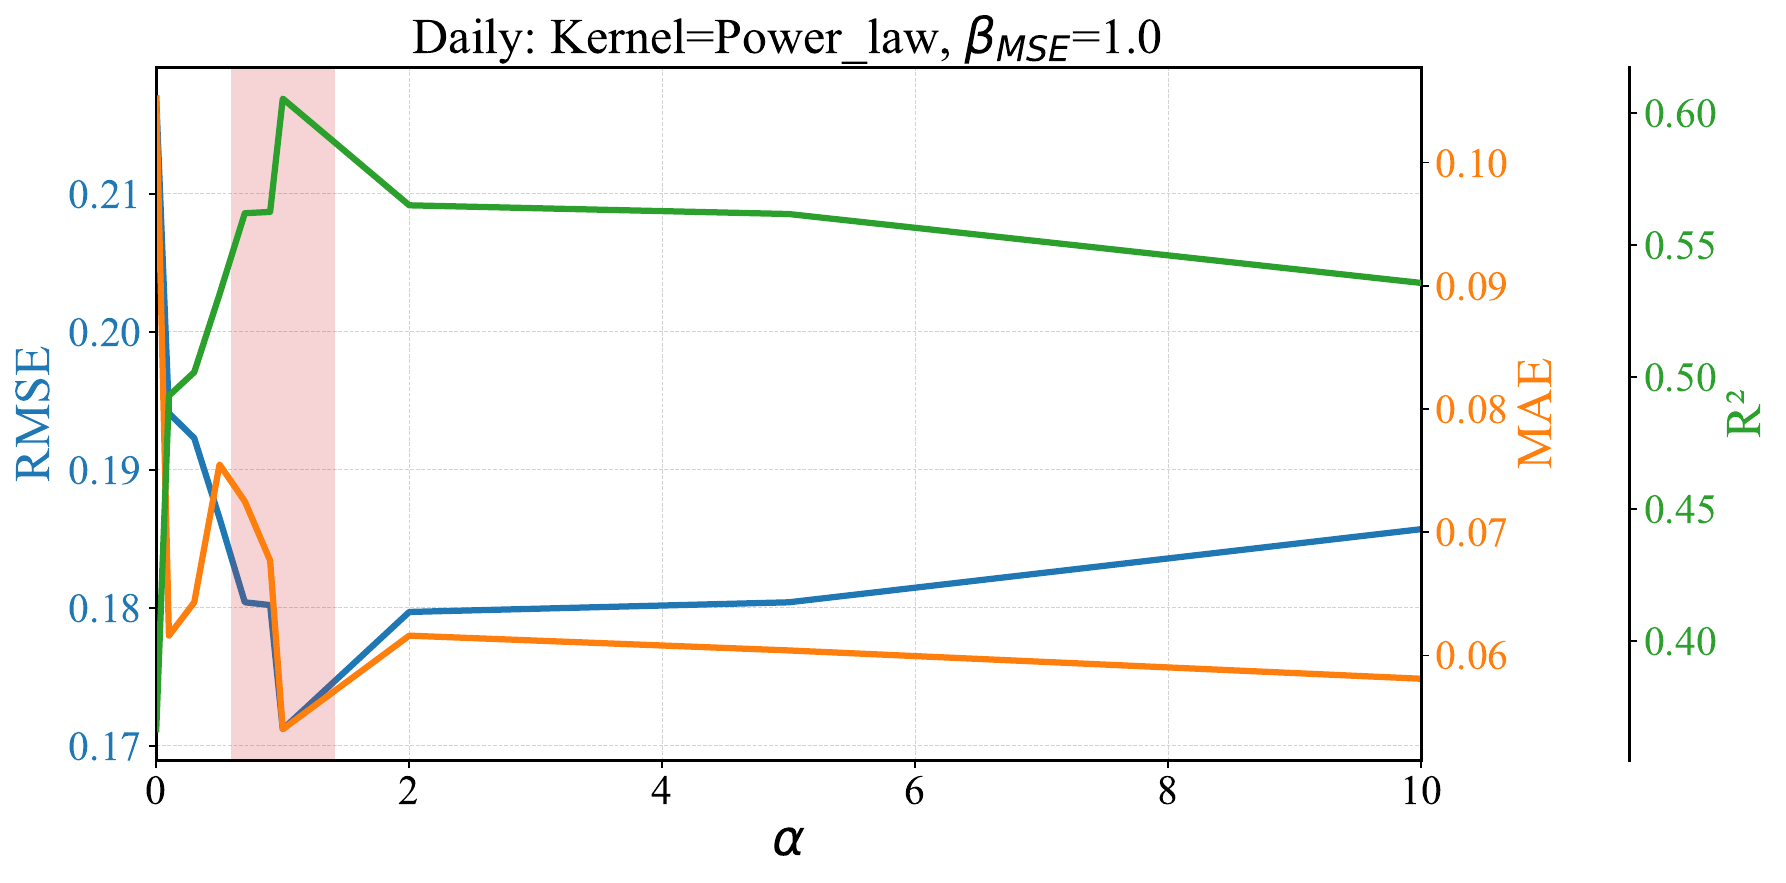}
    \end{minipage}
    \hspace{-6pt}
    \\
% row4
    \begin{minipage}{0.49\textwidth}
        \centering 
        \includegraphics[width=\textwidth]{icml2025/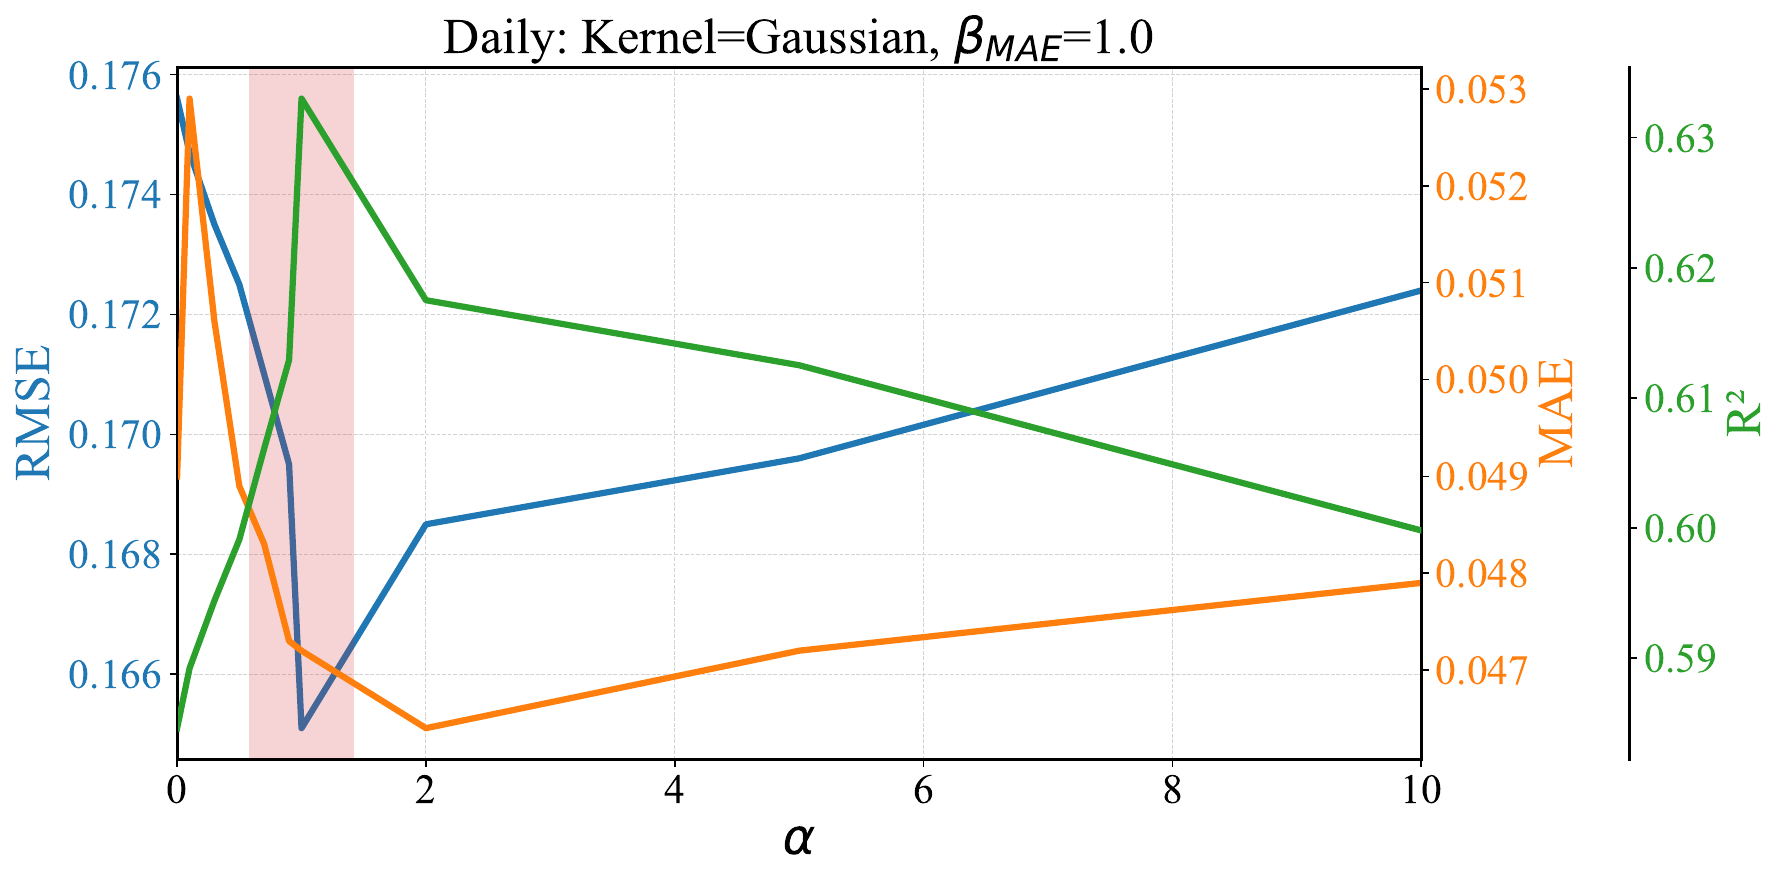}
    \end{minipage}
    \hspace{-6pt}
    \begin{minipage}{0.49\textwidth}
        \centering 
        \includegraphics[width=\textwidth]{icml2025/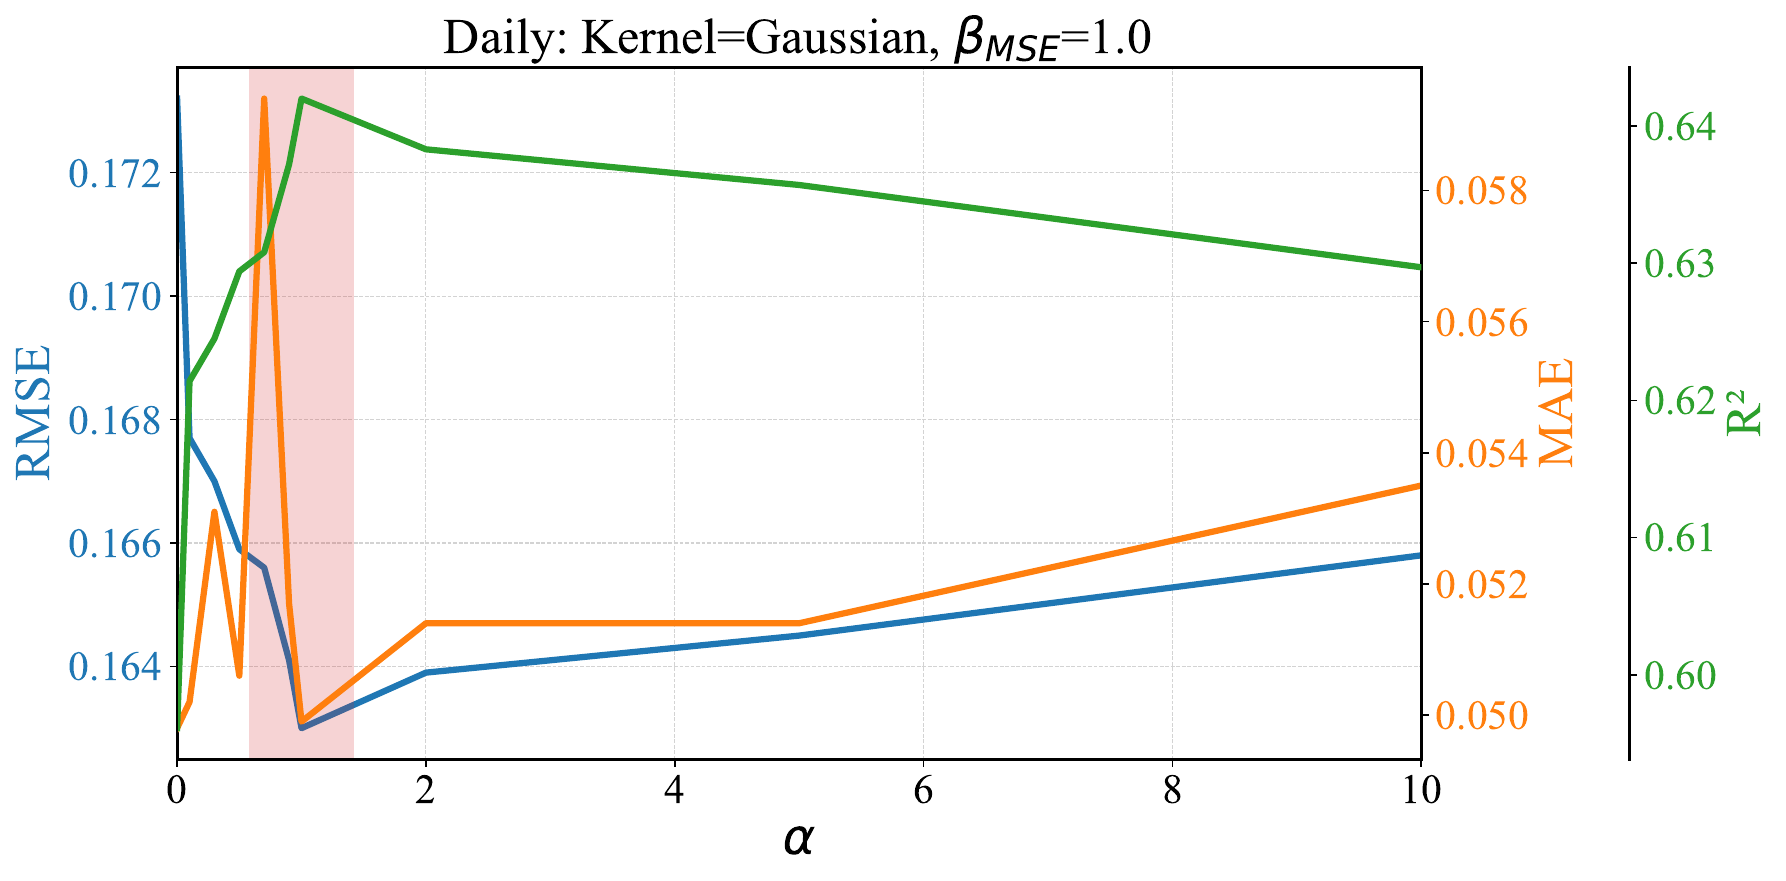}
    \end{minipage}
    \hspace{-6pt}
    \\
    \caption{Comparison of the taper loss parameter \( \alpha \) across different kernel functions and loss types for daily data, evaluating the impact on RMSE, MAE, and \( R^2 \). The parameter \( \beta \) is set to 1.}
    \label{fig_alpha_daily}
\end{figure}

% fig_alpha_hourly
\begin{figure}[!ht]
    \centering
% row1
    \begin{minipage}{0.49\textwidth}
        \centering 
        \includegraphics[width=\textwidth]{icml2025/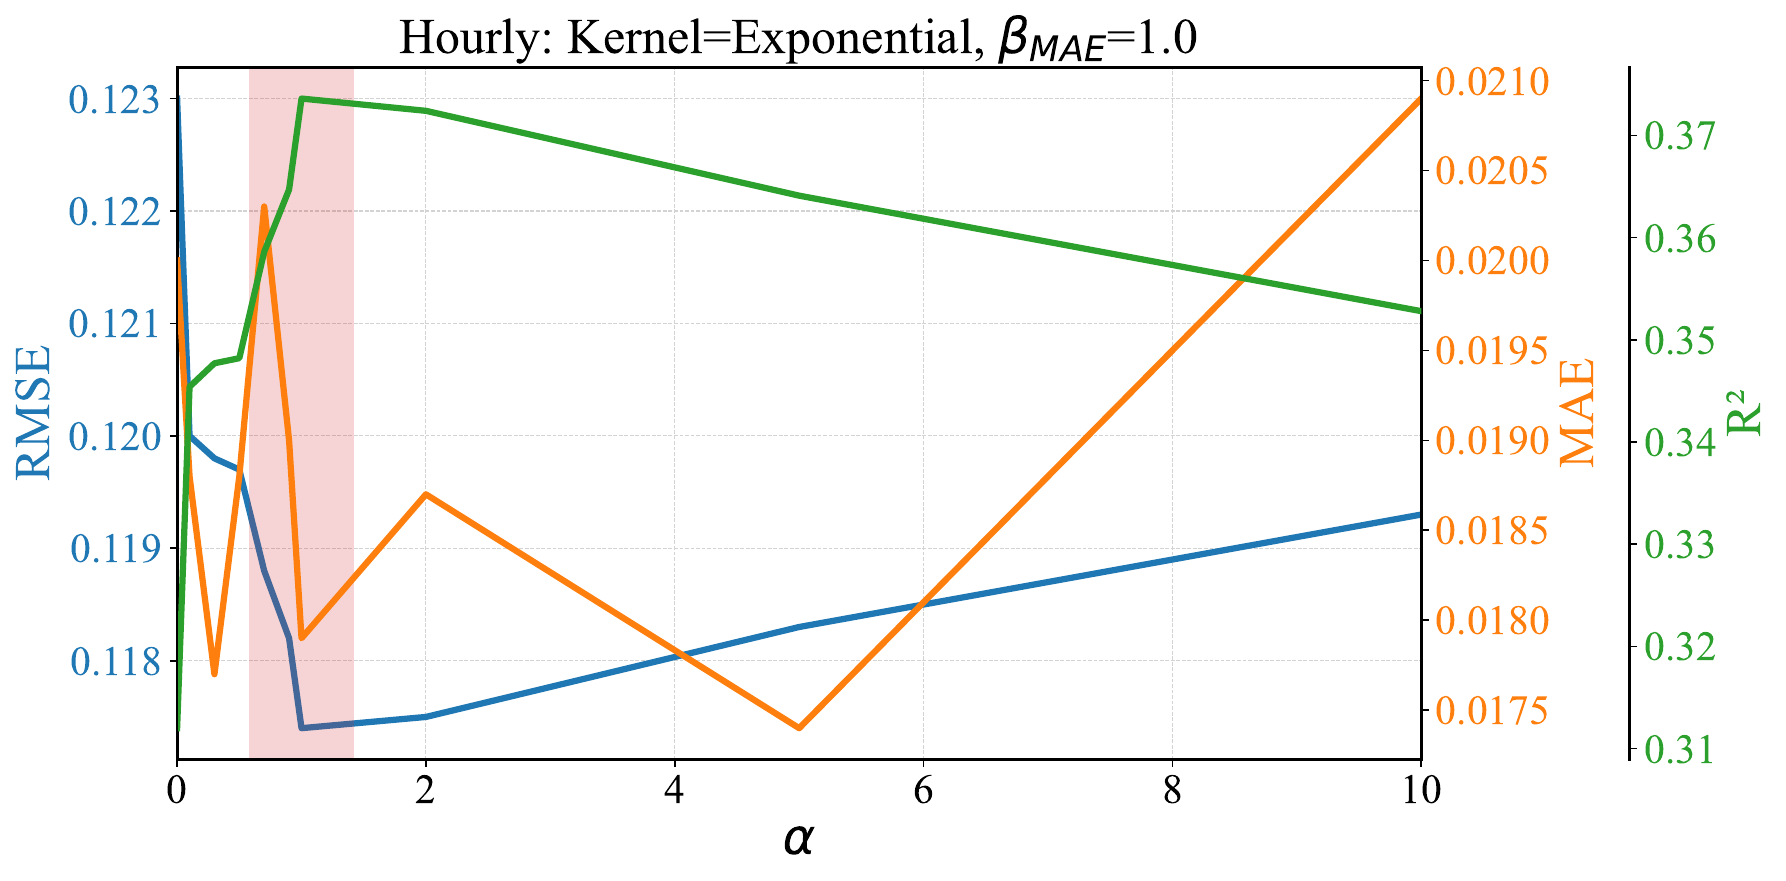}
    \end{minipage}
    \hspace{-6pt}
    \begin{minipage}{0.49\textwidth}
        \centering 
        \includegraphics[width=\textwidth]{icml2025/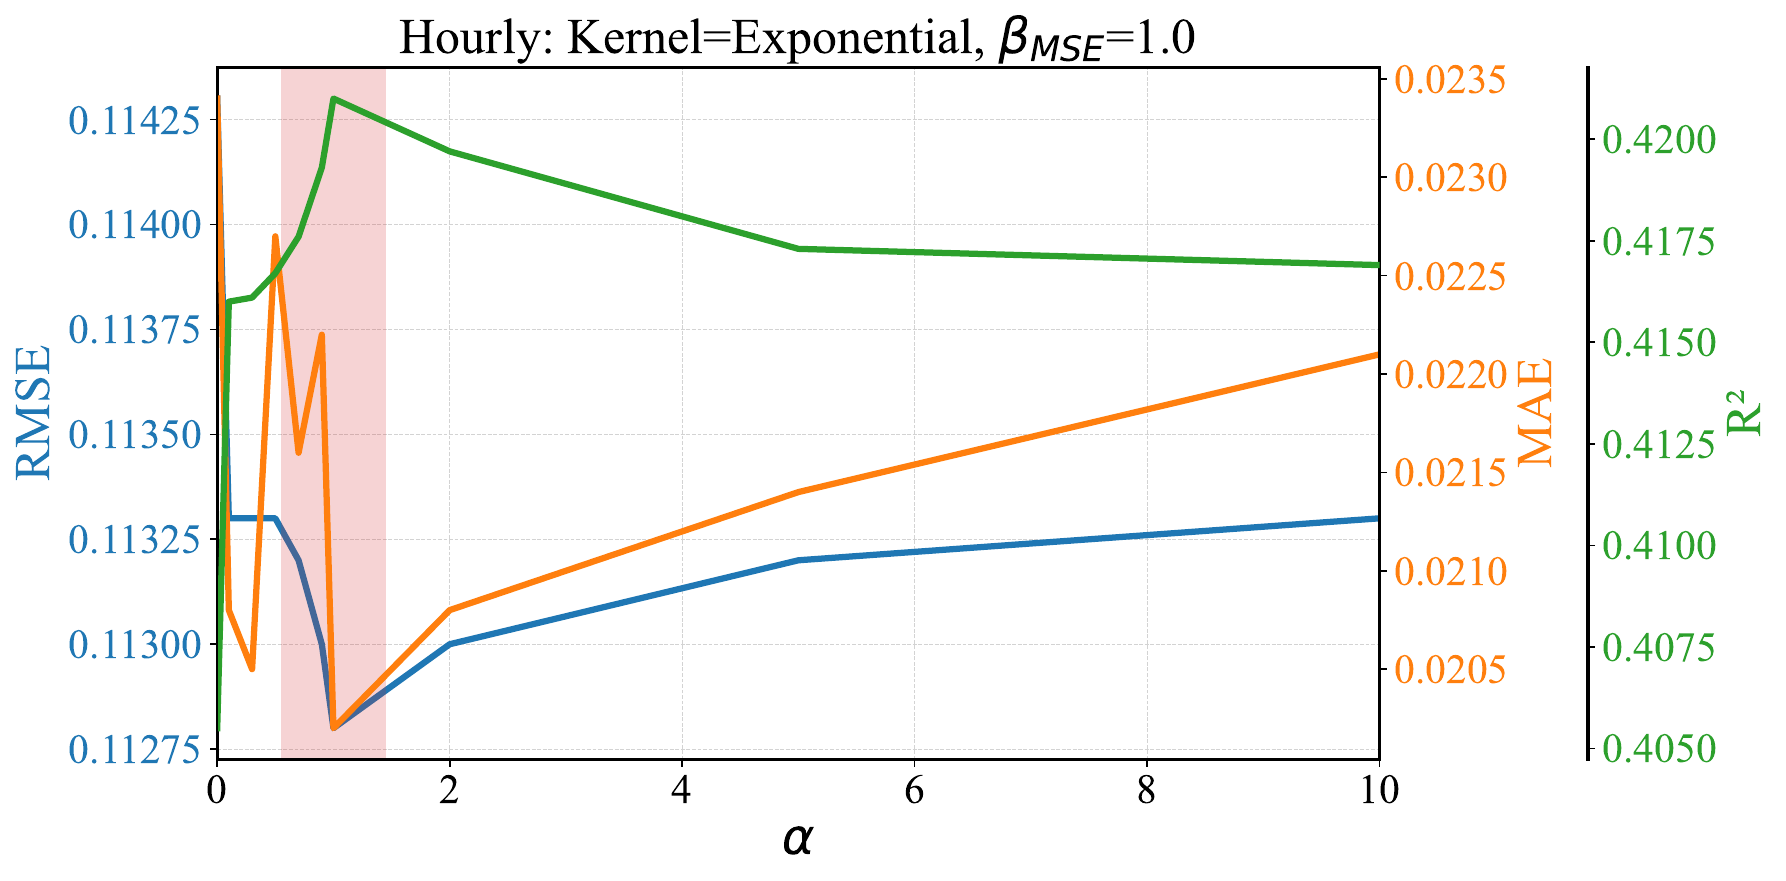}
    \end{minipage}
    \hspace{-6pt}
    \\
% row2
    \begin{minipage}{0.49\textwidth}
        \centering 
        \includegraphics[width=\textwidth]{icml2025/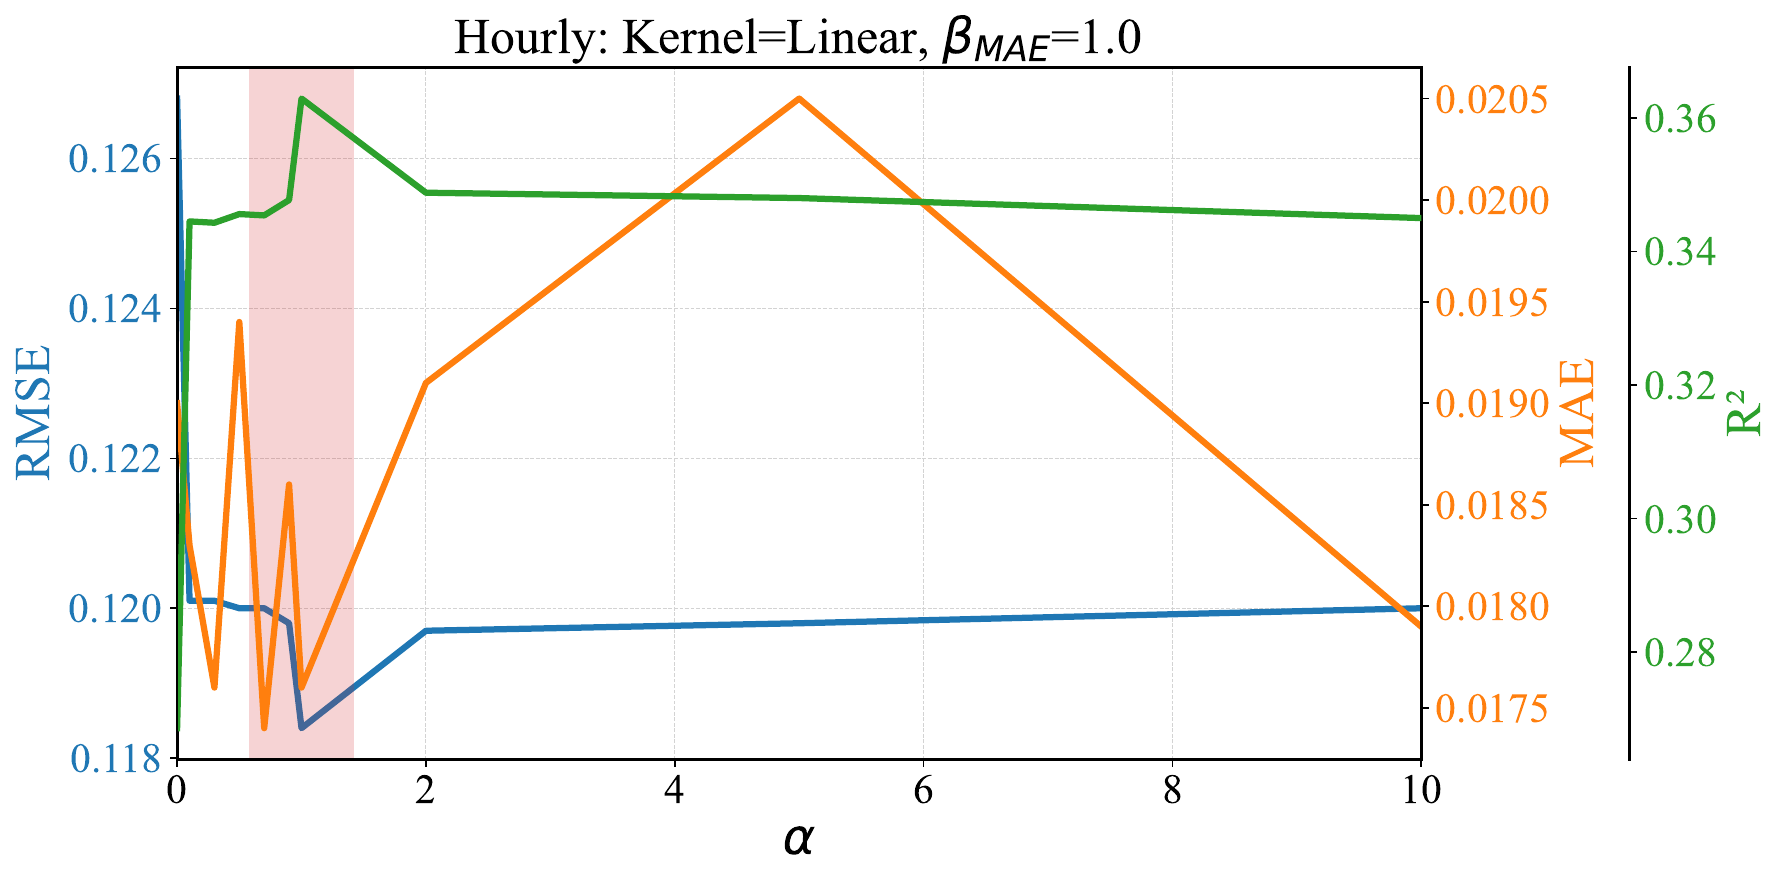}
    \end{minipage}
    \hspace{-6pt}
    \begin{minipage}{0.49\textwidth}
        \centering 
        \includegraphics[width=\textwidth]{icml2025/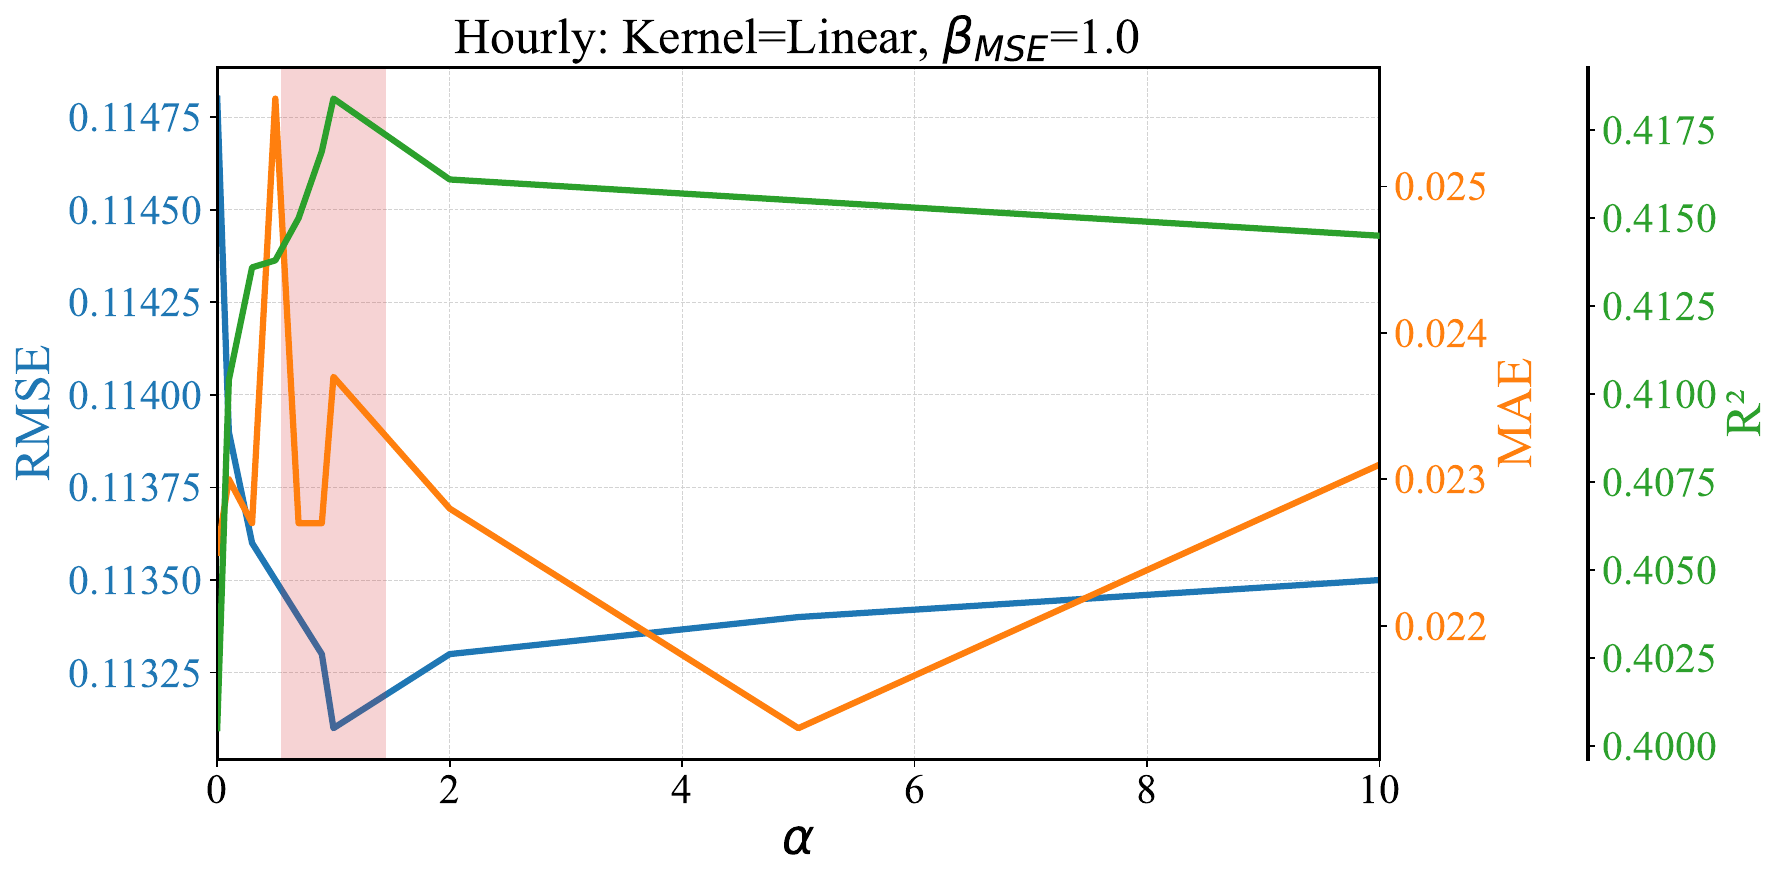}
    \end{minipage}
    \hspace{-6pt}
    \\
% row3
    \begin{minipage}{0.49\textwidth}
        \centering 
        \includegraphics[width=\textwidth]{icml2025/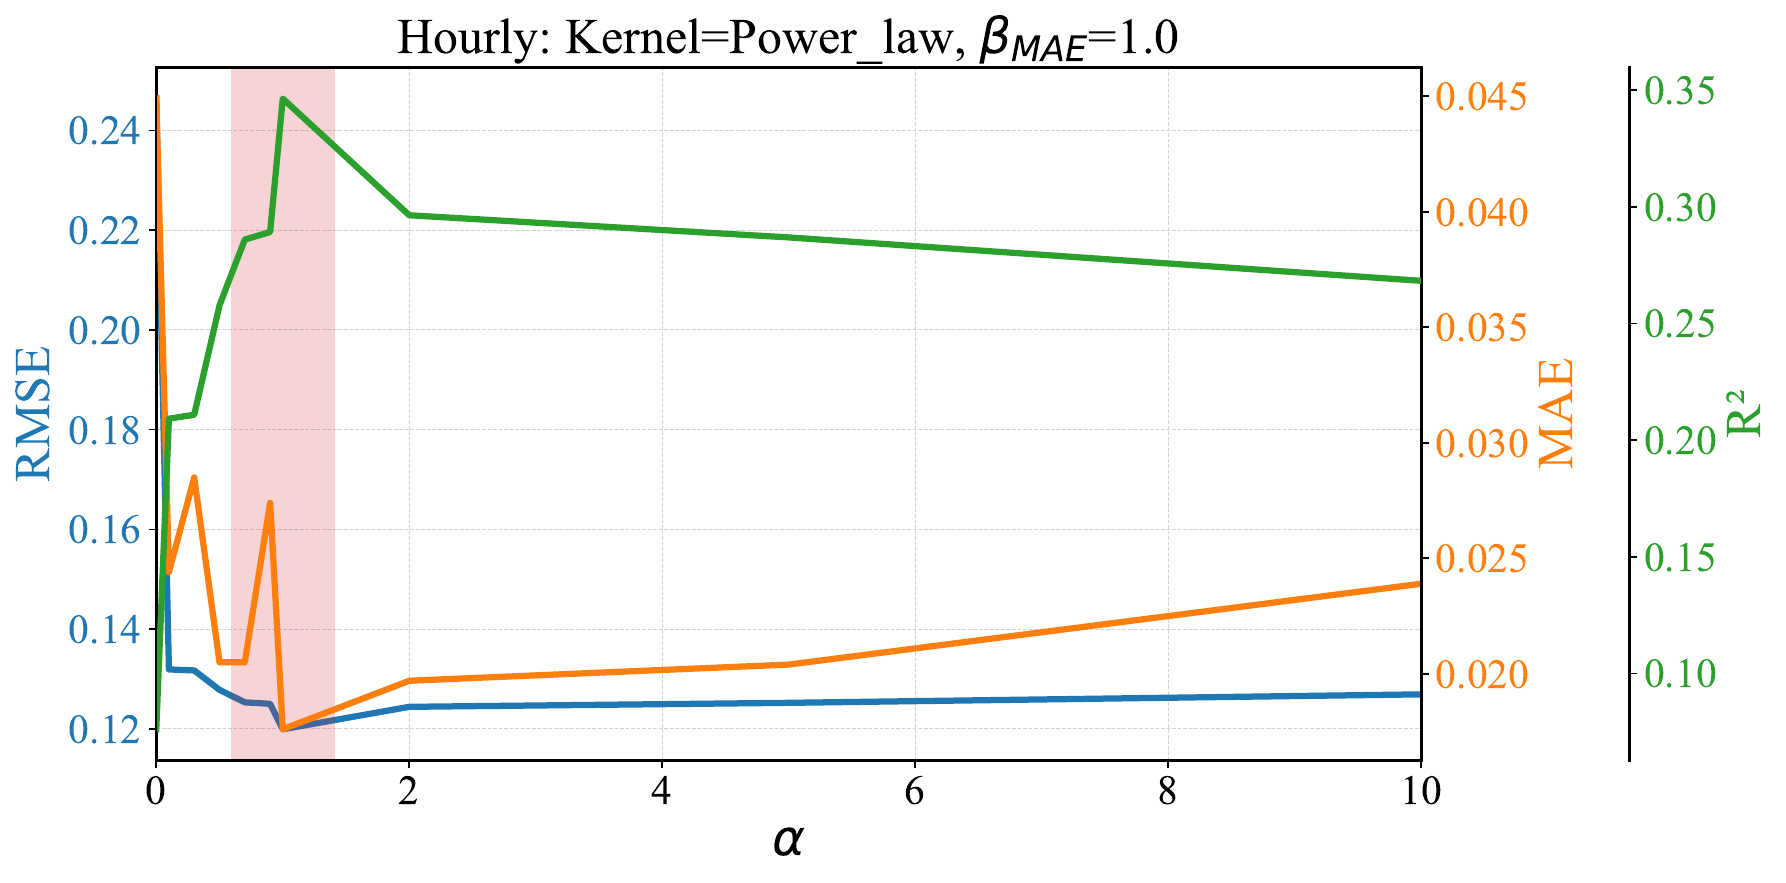}
    \end{minipage}
    \hspace{-6pt}
    \begin{minipage}{0.49\textwidth}
        \centering 
        \includegraphics[width=\textwidth]{icml2025/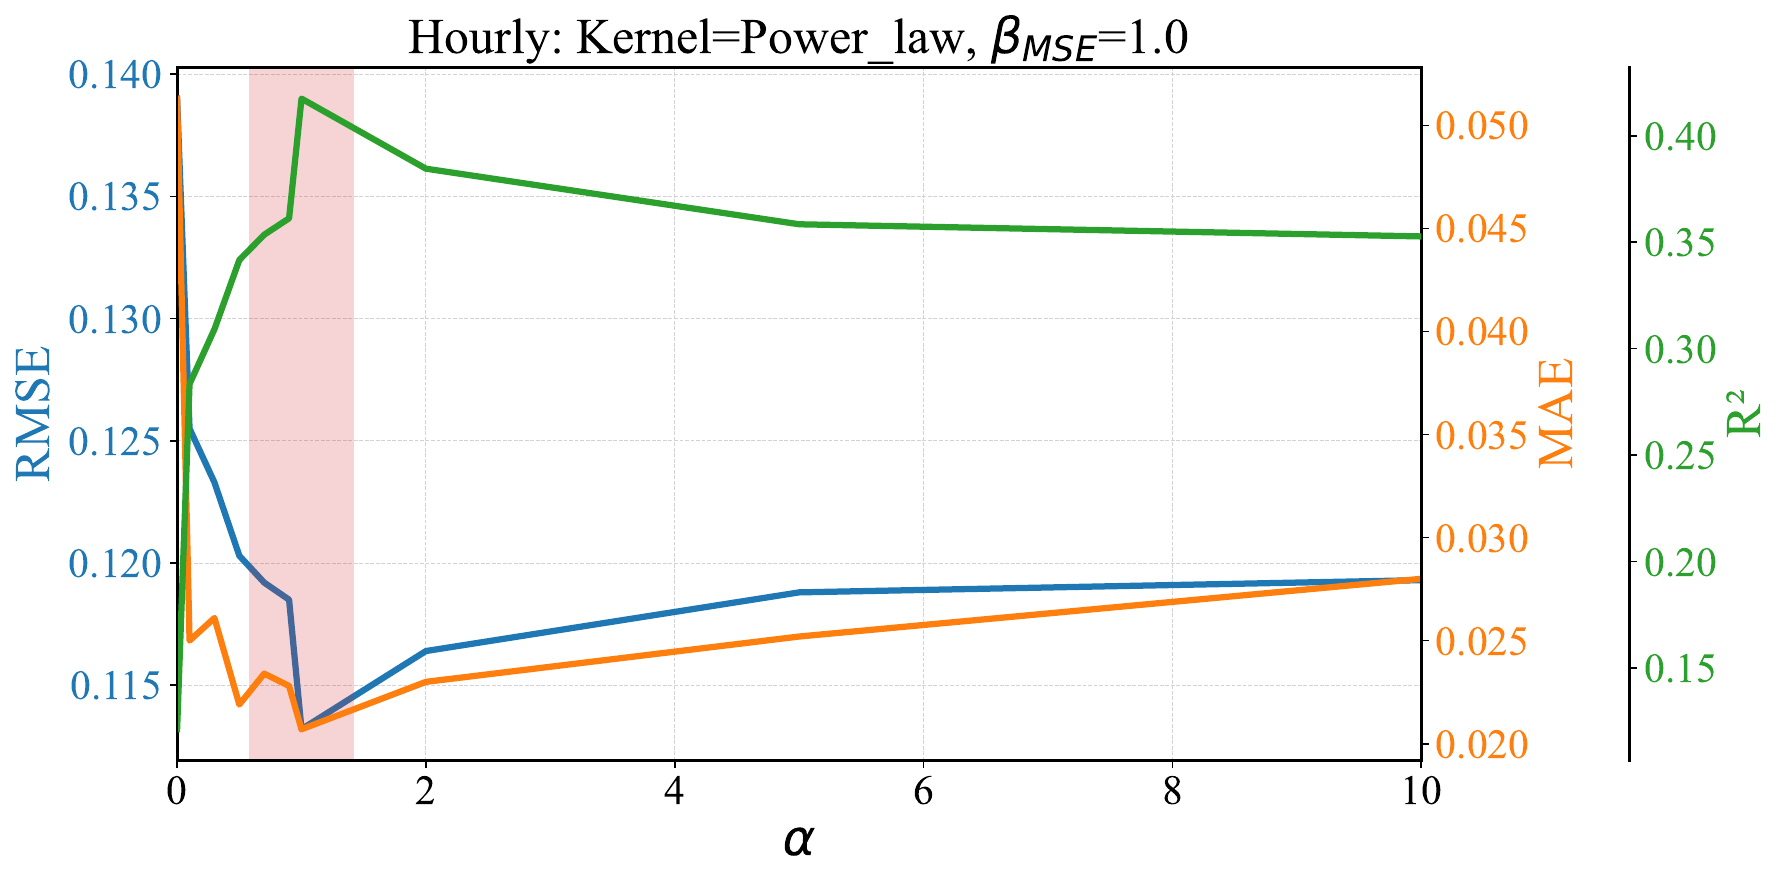}
    \end{minipage}
    \hspace{-6pt}
    \\
% row4
    \begin{minipage}{0.49\textwidth}
        \centering 
        \includegraphics[width=\textwidth]{icml2025/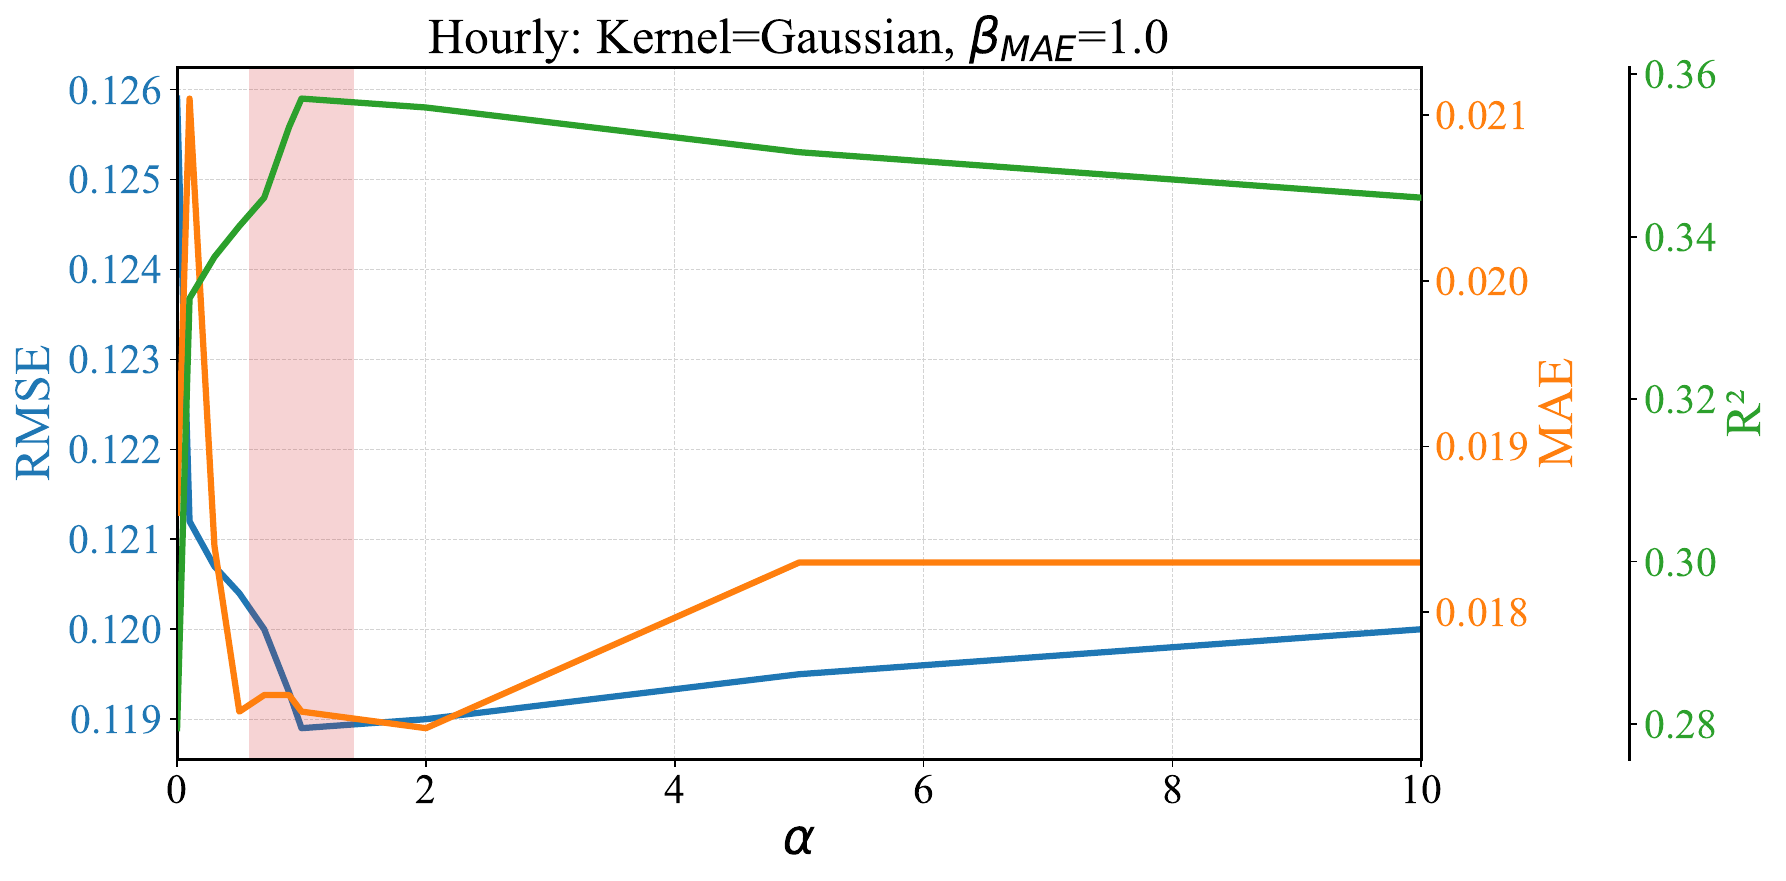}
    \end{minipage}
    \hspace{-6pt}
    \begin{minipage}{0.49\textwidth}
        \centering 
        \includegraphics[width=\textwidth]{icml2025/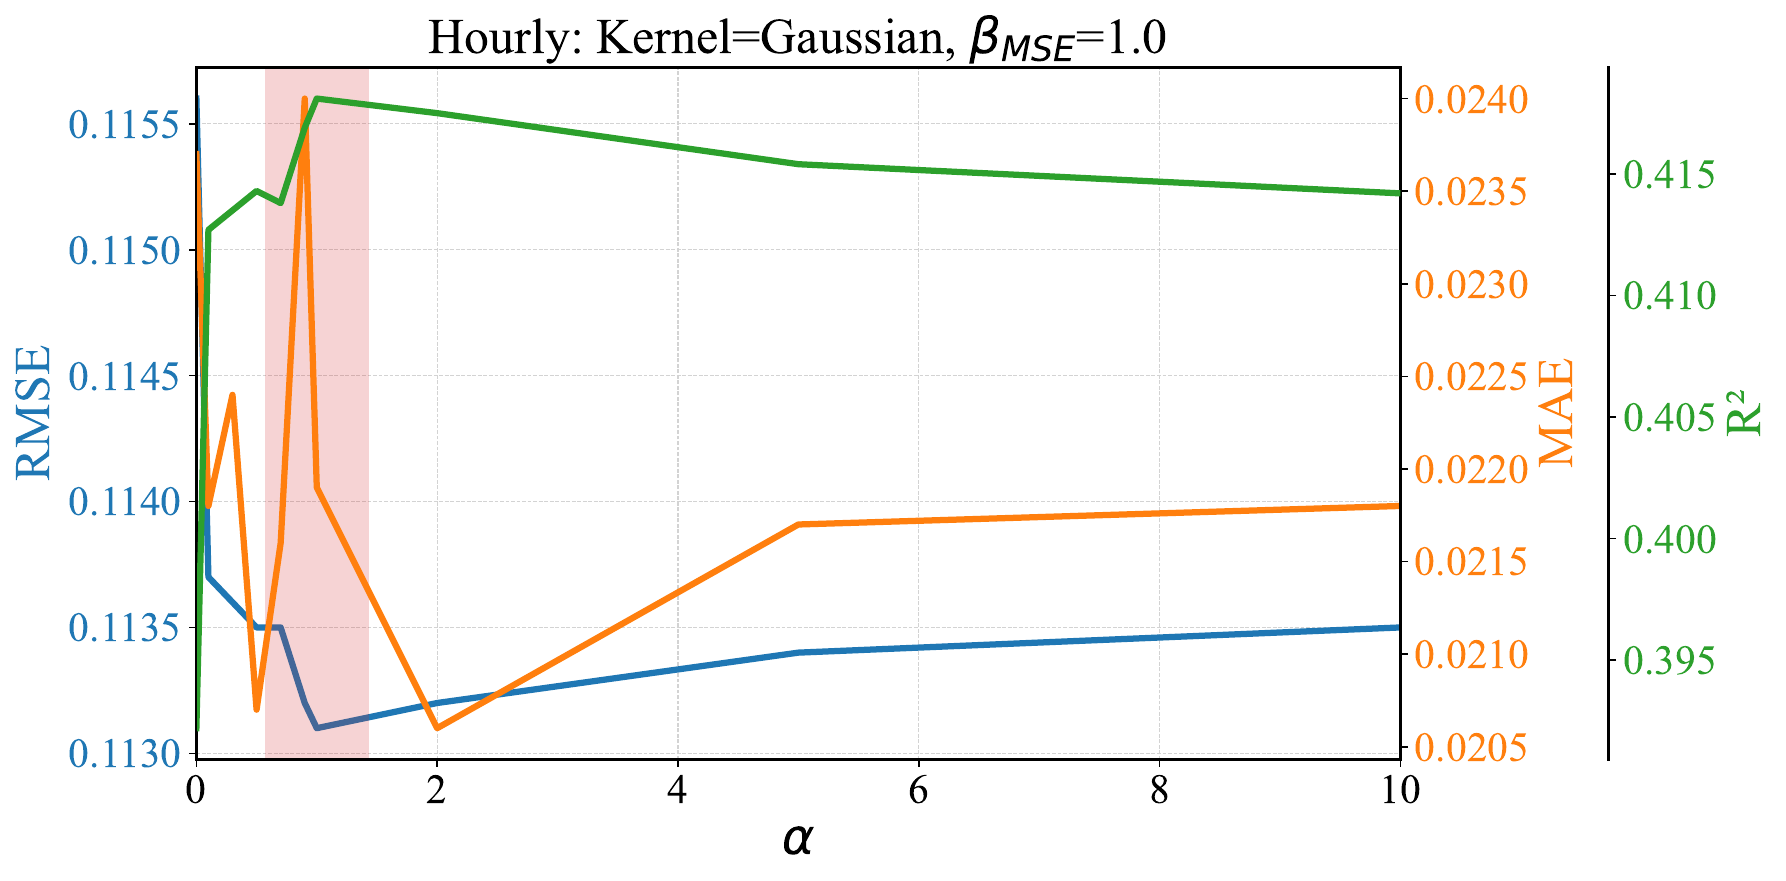}
    \end{minipage}
    \hspace{-6pt}
    \\
    \caption{Comparison of the taper loss parameter \( \alpha \) across different kernel functions and loss types for hourly data, evaluating the impact on RMSE, MAE, and \( R^2 \). The parameter \( \beta \) is set to 1.}
    \label{fig_alpha_hourly}
\end{figure}
